# Supplementary material for: Training-Free Action Recognition and Goal Inference with Dynamic Frame Selection
Source: arXiv:2401.12471 source file (2024-08-28)
Supplement: Supplementary file 1 [file ablation_evidence_selector_additional.tex]

\begin{table}[t]

\centering
\scriptsize

\vspace{5pt}
\resizebox{\textwidth}{!}{
\begin{subtable}
\centering
\begin{tabular}{l|ccccc|ccccc|ccccc}
\toprule 
 \multirow{2}{*}{\textbf{COIN}} & 
 \multicolumn{5}{c|}{\begin{math}\rho\end{math} = 10\%} & 
 \multicolumn{5}{c|}{\begin{math}\rho\end{math} = 30\%} & 
 \multicolumn{5}{c}{\begin{math}\rho\end{math} = 50\%} \\
 
 & \multirow{1}{*}{\footnotesize{S}} & \multirow{1}{*}{\footnotesize{C}} 
 & \multirow{1}{*}{\footnotesize{M}} & \multirow{1}{*}{\footnotesize{B}} & \multirow{1}{*}{\footnotesize{SB}}   
 
 & \multirow{1}{*}{\footnotesize{S}} & \multirow{1}{*}{\footnotesize{C}} 
 & \multirow{1}{*}{\footnotesize{M}} & \multirow{1}{*}{\footnotesize{B}} & \multirow{1}{*}{\footnotesize{SB}} 
 
 & \multirow{1}{*}{\footnotesize{S}} & \multirow{1}{*}{\footnotesize{C}} 
 & \multirow{1}{*}{\footnotesize{M}} & \multirow{1}{*}{\footnotesize{B}} & \multirow{1}{*}{\footnotesize{SB}}\\
 \midrule
w/o ES & 18.3 & 52.8 & 11.4 & 23.0 & 41.9 
& 21.0 & 63.2 & 12.7 & 26.7 & 46.1
& 22.0 & 68.2 & 13.2 & 27.8 & 47.7
\\

\textbf{with ES}& \textbf{20.4} & \textbf{62.6} & \textbf{12.5} & \textbf{27.2} & \textbf{45.0}
& \textbf{23.0} & \textbf{71.4} & \textbf{13.7} & \textbf{30.4} & \textbf{49.6}
& \textbf{25.1} & \textbf{76.7} & \textbf{14.3} & \textbf{31.6} & \textbf{51.5}
\\

 \bottomrule
\end{tabular}

\end{subtable}
}

(a) Goal inference on COIN dataset

\vspace{5pt}
\begin{subtable}
\centering
\begin{tabular}{l|ccccc}
\toprule 
 \multirow{2}{*}{\textbf{ActivityNet}} & 
 \multicolumn{5}{c}{\begin{math}\rho\end{math} = 100\%} \\

 & \multirow{1}{*}{\footnotesize{S}} & \multirow{1}{*}{\footnotesize{C}} 
 & \multirow{1}{*}{\footnotesize{M}} & \multirow{1}{*}{\footnotesize{B}} & \multirow{1}{*}{\footnotesize{SB}}\\
 \midrule
w/o ES & 21.2 & 79.6 & 12.7 & 22.3 & 57.4 \\

\textbf{with ES}& \textbf{24.0} & \textbf{94.0} & \textbf{14.7} & \textbf{28.8} & \textbf{61.0} \\
 \bottomrule

\end{tabular}
\end{subtable}%

(b) Action recognition on Activitynet dataset
    
\centering

\caption{Ablation study of the evidence selector (ES) component on COIN and ActivityNet.}
\label{tab:ablation_evidence_selector_additional}
\end{table}
